# Supplementary material for: On the applicability of single-spacecraft interferometry methods using electric field probes
Source: arXiv:2111.10288 ancillary file (2022-02-18)
Supplement: Supplementary file 1 [file Supporting_information.pdf]

*Journal of Geophysical Research: Space Physics*

Supporting Information for

**On the applicability of single-spacecraft interferometry methods using electric field probes**

K. Steinvall[1,2], Yu. V. Khotyaintsev[1], D. B. Graham[1]

[1]Swedish Institute of Space Physics, Uppsala, Sweden
[2]Space and Space Plasma Physics, Department of Physics and Astronomy, Uppsala University, Uppsala, Sweden

## Contents of this file

Figures S1 to S3

## Introduction

Figure S1 shows the $(\theta, \varphi)$ surfaces for the ratio of the estimated and prescribed speed $v/v'$ (left column) and the angle between the estimated and prescribed velocity vectors $\alpha$ (right column) for different values of $L_\perp/L_\parallel$ when spacecraft potential effects are ignored. Figure S2 shows similar surface plots for different values of $n$, with $\xi_{1-4} = 0.05$ and $\xi_{5,6} = 0.06$, when $L_\parallel = 50$ m and $L_\perp/L_\parallel = 50$. Figure S3 has the same format as S2, except with $\xi_{1-4} = 0.167$ and $\xi_{5,6} = 0.180$.

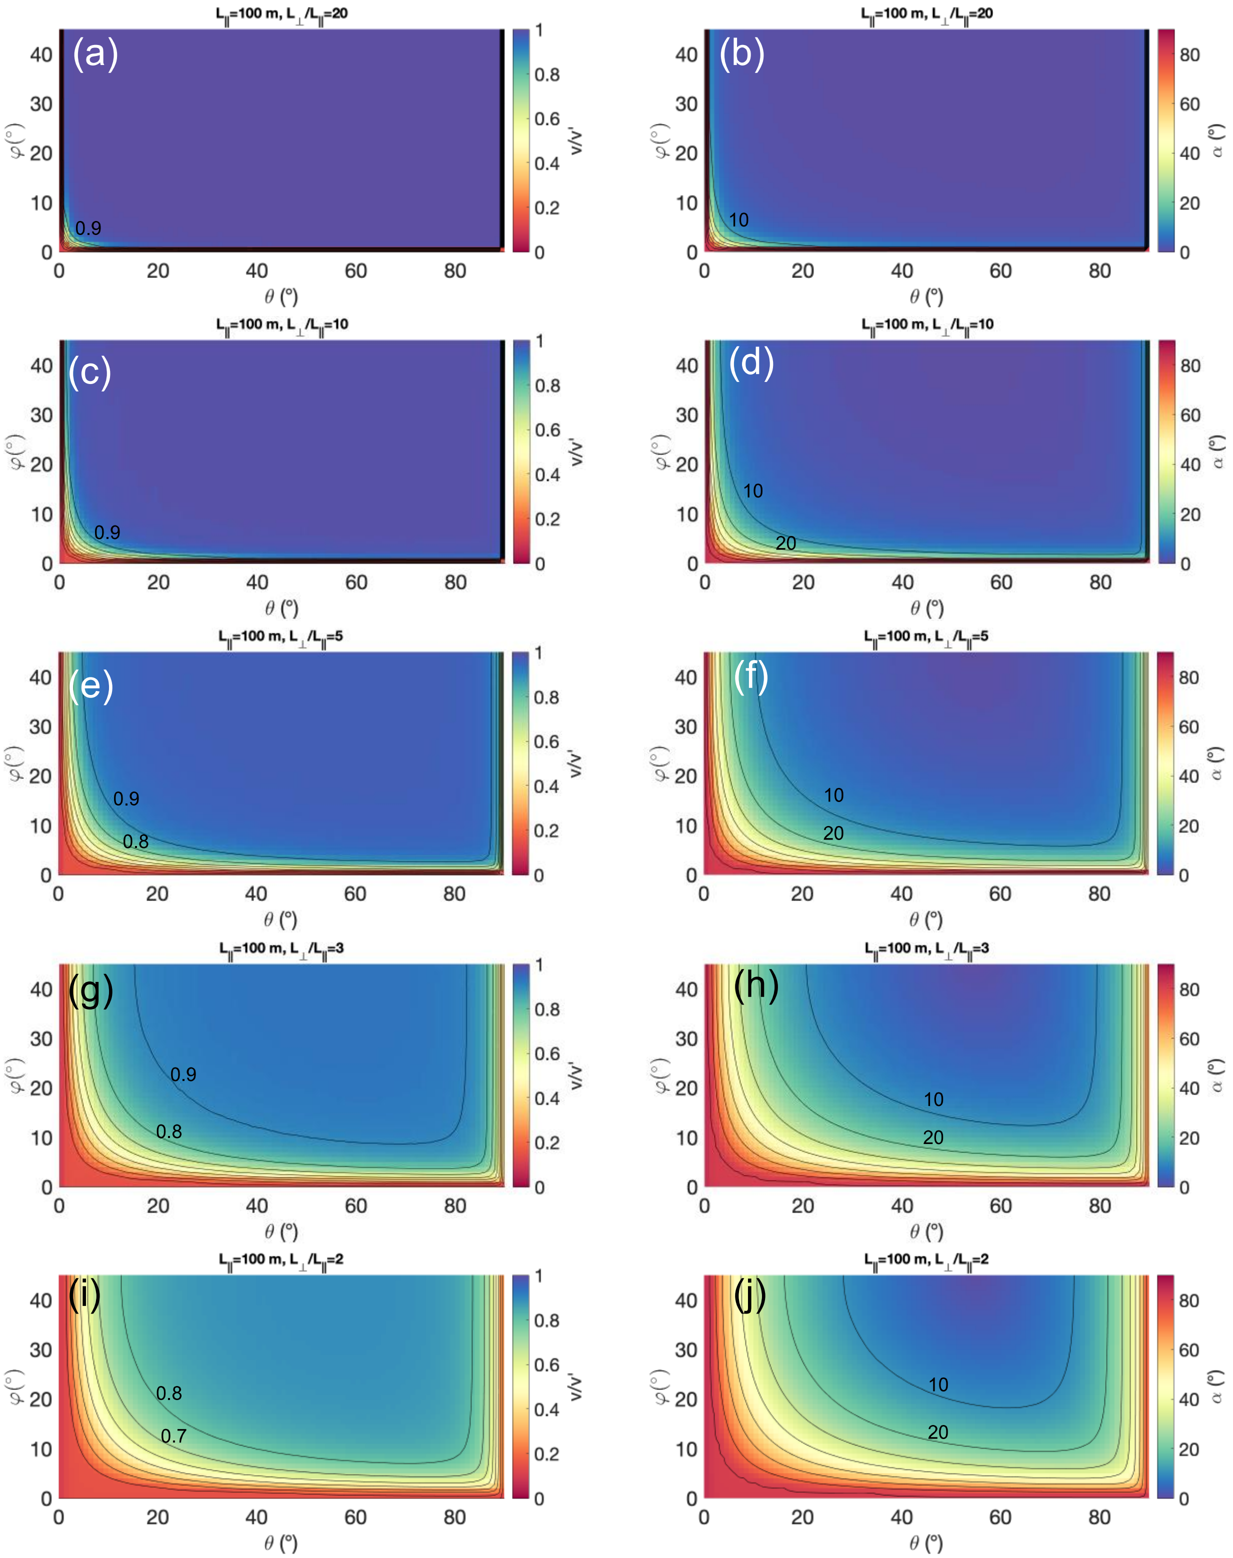


Figure S1. Left column: $v/v'$ as a function of $\theta$ and $\varphi$ for different values of $L_{\perp}/L_{\parallel}$. Right column: Angle $\alpha$ between $\boldsymbol{v}$ and $\boldsymbol{v}'$ as a function of $\theta$ and $\varphi$ for different values of $L_{\perp}/L_{\parallel}$.

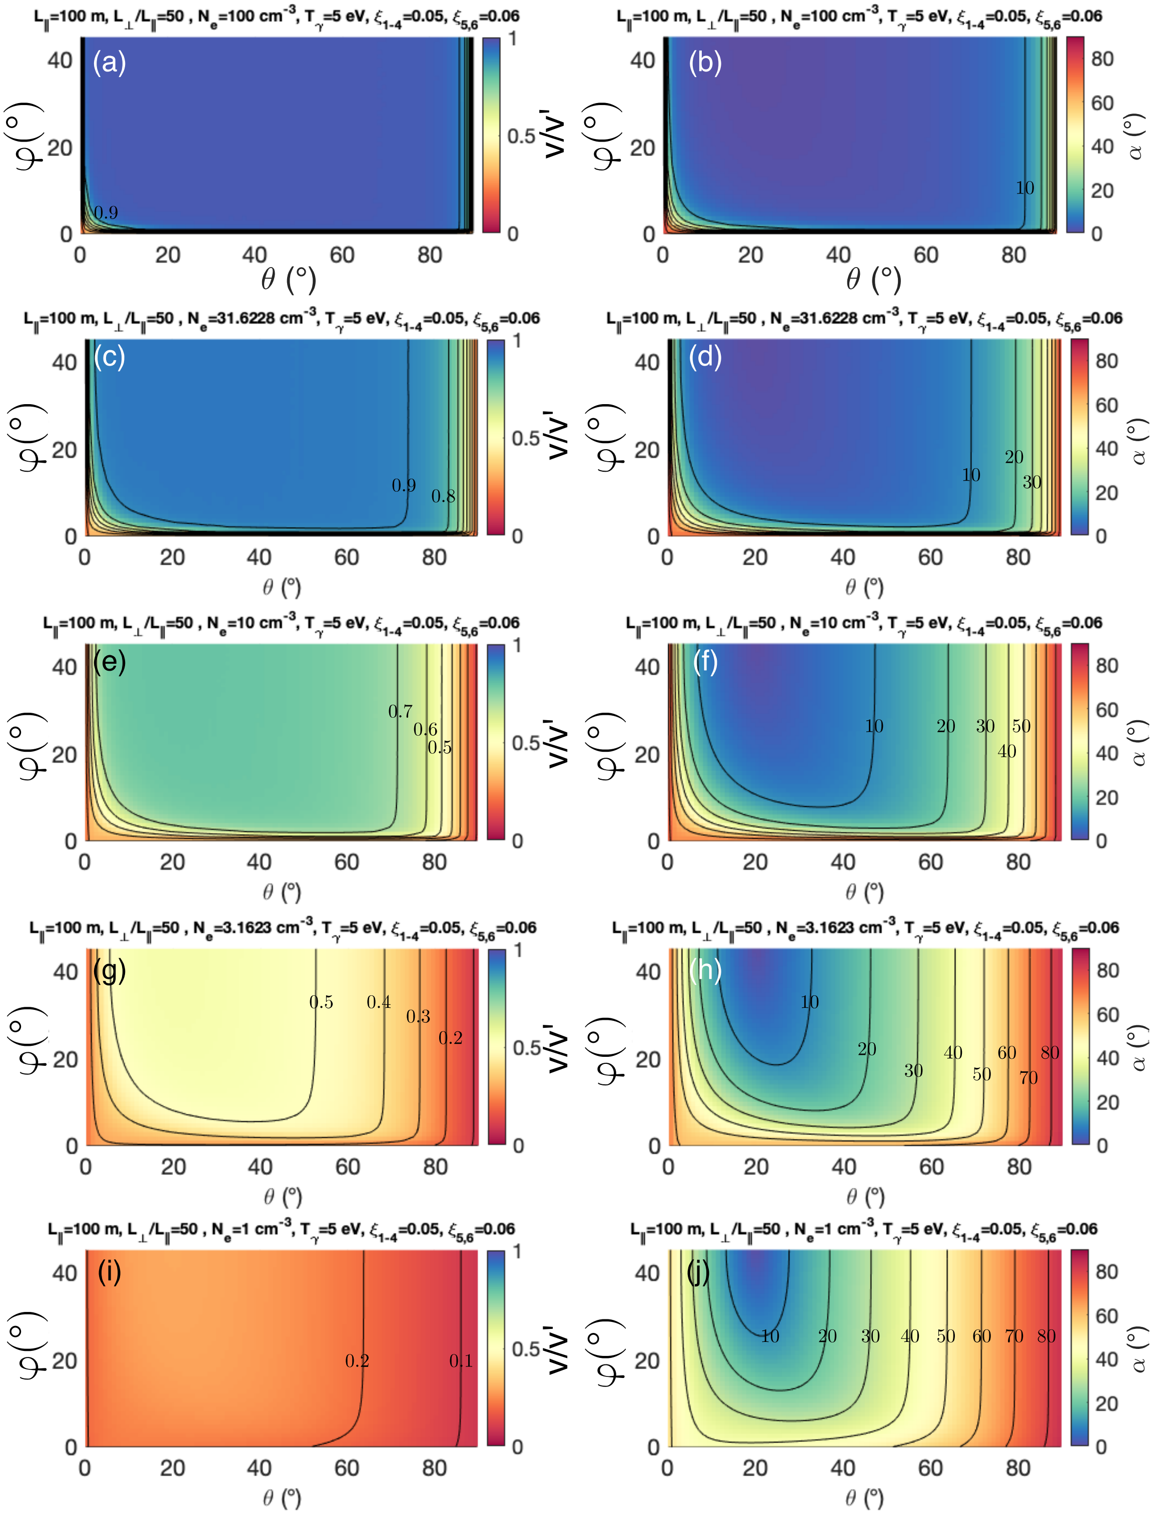


Figure S2. $v/v'$ (left column) and $\alpha$ (right column) as a function of plasma density $n$ for $L_{\parallel} = 100$ m, $L_{\parallel}/L_{\perp} = 50$, $\xi_{1-4} = 0.05$ and $\xi_{5,6} = 0.06$.

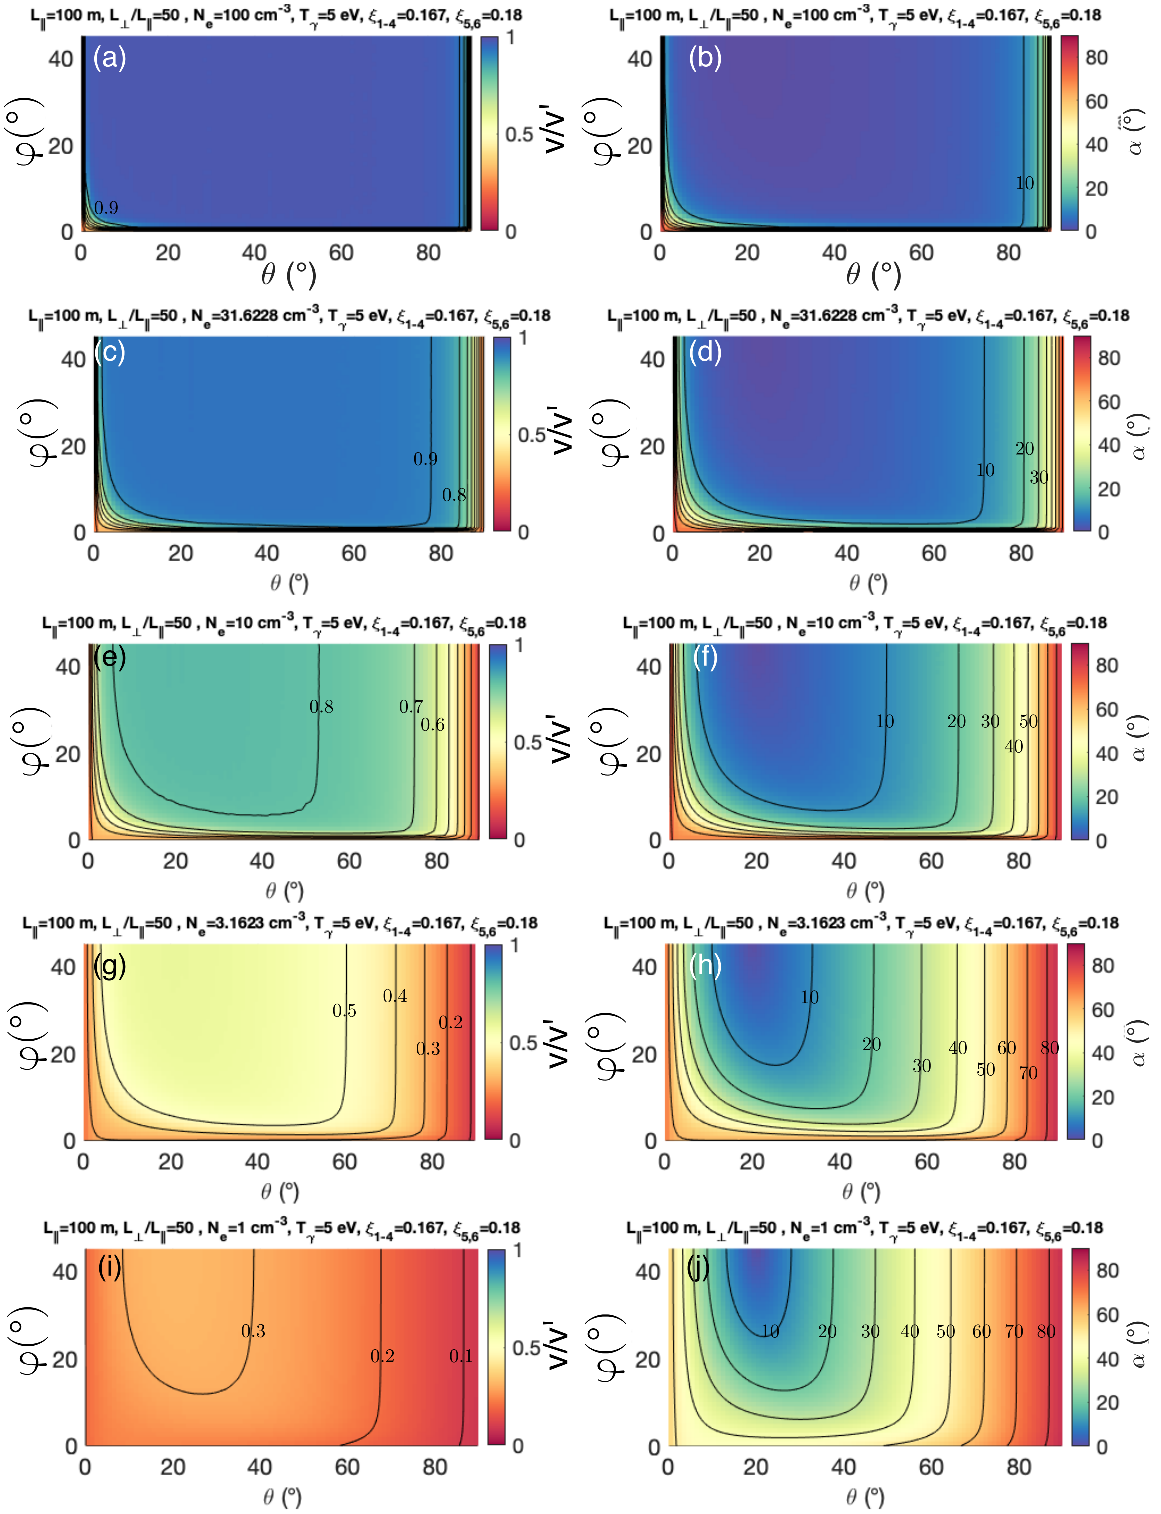


Figure S3. Same format as Fig. S2, except with $\xi_{1-4} = 0.167$ and $\xi_{5,6} = 0.18$.
